# Supplementary material for: HTML papers on arXiv -- why it is important, and how we made it happen
Source: arXiv:2402.08954 ancillary file (2024-02-14)
Supplement: Supplementary file 1 [file Slide-deck-Japanese-version-of-arXiv-DEIMS-2024.pdf]

# HTML papers on arXiv

arXivにおけるHTML論文

Why it's important, and how we make it happen

その重要性和実現までの過程

# arXiv's Importance in Math and Science

## 数学と科学におけるarXivの重要性

- arXiv ([arxiv.org](https://arxiv.org)) is the world's oldest and largest scientific preprint server

arXiv は世界で最初で最大の未出版科学論文のサーバー

- Started in 1991

平成3年から運営

- Presently housing nearly 2.4 million articles

現在240万件の記事を採集

- Growth is accelerating

成長が加速している

Total number of submissions as of December 9, 2023 = 2,380,492.

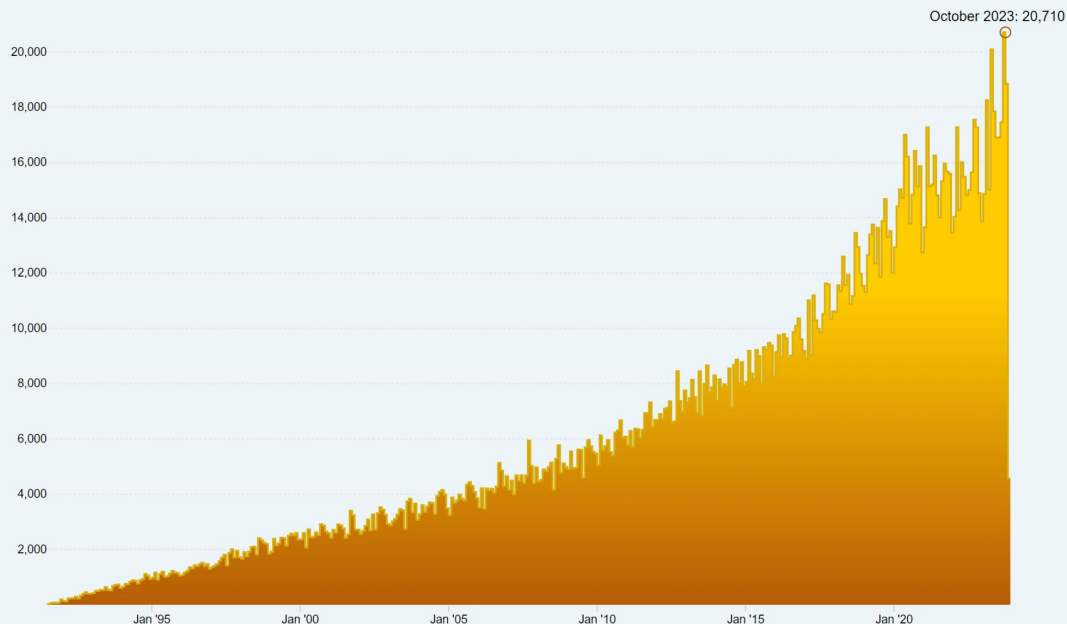

# arXiv's Importance in Math and Science

- In many fields of Physics, Math, and especially Computer Science, cutting edge research is first made available on arXiv. Examples:
  - LLM research ([OpenAI](#), [Deepmind](#), etc.)
  - [LIGO](#) (Gravity wave research; [2017 Nobel Prize in physics](#))
  - Proofs of famous theorems ([Grisha Perelman](#))
- While most papers posted to arXiv are eventually published in journals, in some fields research is often made available only on arXiv
- And even for work subsequently published in journals, early posting to arXiv enables scientists to more rapidly incorporate shared results into new research

## 数学と科学におけるarXivの重要性

- 物理 数学 特に情報学の数々の分野で、最新の研究は arXiv 上で最速にアクセス／利用できます  
例:
  - LLM 研究 ([OpenAI](#), [Deepmind](#), 等.)
  - [LIGO](#) (重力波研究;平成29年 ノーベル物理学賞)
  - 著名な定理の証明 ([Grisha Perelman](#))
- arXiv に投稿された論文の多くは最終的にジャーナル等に掲載されますが、一部の分野では論文が arXiv でのみ利用可能になる場合も珍しくありません
- また、その後ジャーナルに掲載された研究でも、arXiv に早期に投稿することで、研究者は提供された研究をより迅速に新しい研究に取り入れることができます

## arXiv and accessibility

- Over the past few years, arXiv has made good progress in making <https://arxiv.org> accessible according to [W3C WAI guidelines](#)
- While this allows people with disabilities to more easily access papers, they often cannot read them
- Because arXiv's papers are available almost exclusively in PDF format, which is not, in general, accessible

## arXiv とバリアフリー

- 過去数年にわたって、arXiv は W3C WAI ガイドラインに従って <https://arxiv.org> をバリアフリーにするという点で着実な進歩を遂げてきました
- 障害者がより簡単に論文にアクセスできるようになりましたが、多くの場合、論文内容を読むことができません
- arXiv の論文はほぼ PDF 形式でのみ入手可能であり、内容のアクセスはバリアになっています

# PDF limitations - layout

- PDF was originally designed as a digital representation of a printed page
- There is often a mismatch between the paper's geometry and the screen being used to view it
- Zooming in to enlarge the text will often require horizontal scrolling
- “Responsive Design” and reflow are not natural parts of PDF
- Adobe is attempting to address these issues with features like “Liquid Mode”
  - But Liquid Mode is presently mobile-only, and Adobe proprietary
  - Not clear if this retroactive reinterpretation of PDF document layout will work well in all cases
- Improvements in layout and reflow help everyone – not just people with impairments
  - Makes it easier to read papers on mobile devices

# PDF の制約 - レイアウト

- PDF は原来、印刷されたページのデジタル表現として設計されています
- 紙の形状とそれを表示するために使用される画面の間に不一致が多々あります
- テキストを拡大するためにズームインすると、多くの場合、水平スクロールが必要になる
- 「レスポンシブ デザイン」とリフローは PDF の設計思想に含まれていません
- アドビは「リキッドモード」などの機能でこれらの問題に対処しようとしています
  - ただし、リキッド モードは現時点ではモバイル専用で、アドビ独自のものです
  - PDF ドキュメント レイアウトのこの遡及的な再解釈がすべての場合にうまく機能するかどうかは不明
- レイアウトとリフローの改善は、障害者対策、バリアフリーに限らず、全ての利用者に利益があります
  - 携帯デバイスで論文を読みやすくなります

# PDF Structure Limitations PDF の文書構成の制約

- The original structure of the paper, that screen readers often depend on for navigation is typically lost
  - Section headings, captions, links, etc. are reduced to typographic elements like font changes and positioning instructions
  - Mathematical notation in PDF is reduced to symbols and positioning directives
- Adobe introduced tagged PDF in recent years to improve this situation
- But the vast majority of PDF documents in the world are not tagged, tool support has lagged, and there's still the reflow issue
- Again Adobe is attempting to address these issues with features like Tagged PDF
  - arXiv's pipeline from TeX -> PDF currently has poor support for tagged PDF (waiting for the core LaTeX team to give us a solution here)
  - Tagged PDF also has a weak solution for math - display the math as an image and describe the formula in the alt-text for screen readers
- 論文の文書構成情報が失われ、スクリーン読み取りアプリがナビゲーションをできなくなる
  - セクションの見出し、キャプション、リンクなどは、フォントの変更や位置の指示などの印刷要素に変換される
  - PDF の数学的表記はシンボルと位置決め命令に変換される
- アドビはこの状況を改善するために、近年タグ付き PDF を導入しました
- しかし、世界中の PDF ドキュメントの大部分はタグ付けされておらず、ツールのサポートも遅れており、リフローの問題も依然として残っています
- 繰り返しですが、アドビはタグ付き PDF などの機能でこれらの問題に対処しようとしています。
  - TeX -> PDF からの arXiv のパイプラインは現在タグ付きPDFを十分にサポートしていません(LaTeX 核チームがここで解決策を提供してくれるのを待っています)
  - タグ付き PDF は、数式の対処に問題点がある。数学を画像として表示し、スクリーンリーダーの代替テキストで数式を表現する

# HTML is a better solution

- Designed from the start to render on many devices, arbitrary geometries
- When used correctly preserves structure and intent of the document
- A lot of work has been done to make HTML accessible
- A rich “marketplace” of assistive technologies to make HTML content accessible
- For most people HTML is the gateway to all the content the WWW has to offer
- But ...
- There's a substantial body of scientific work online available only in PDF format
- Converting PDF content to HTML is challenging, in spite of some interesting work allen.ai has done in this area ([Paper to HTML | Allen Institute for AI](#))
  - Because structure, once lost, is difficult to reconstruct

# HTMLで解決可能になること

- 多くのデバイス、任意の領域でレンダリングできるように最初から設計されています
- 正しく使用すると、文書の構造と意図が保持
- HTML をバリアフリーにするための規格と実現への数々の努力が払われています
- HTML コンテンツにアクセスできるようにする支援技術のマーケットが豊富であること
- ほとんどの人にとって、HTML は WWW が提供するすべてのコンテンツへの入り口です
- しかし ...
- オンライン上には、PDF 形式でのみ利用できる科学的成果のかなりの量があります
- allen.ai がこの分野でいくつかの興味深い研究を行っていますが、PDF コンテンツを HTML に変換するのは困難 ([Paper to HTML | Allen Institute for AI](#))
  - 一度失われた構造を再構築するのは難しい

# HTML has a strong ecosystem HTMLの豊富な環境

- Because use of the World Wide Web has become fundamental to human existence, a great deal of effort has been expended to make the web accessible
- There's a vibrant ecosystem of screen readers for HTML web pages
- The “open-source” structure of HTML enables add-ins to easily change page appearance to aid visually impaired and people with dyslexia
- “Dark mode” is now widely supported for those with light sensitivities
- Modern web browsers now build-in useful features like language translation
  - Which is an “accessibility” improvement for a class of users
- Search engines function better on HTML content
  - Although the situation for finding content in PDFs is much better now than the early years
- Text harvesting is easily from HTML documents
  - arXiv's corpus is a substantial part of nearly all the Large Language Models today
- ウェブの使用は生活の基礎条件となってきたため、ウェブをバリアフリーにするために多大な努力が費やされてきました
- **HTML Web** ページ用のスクリーンリーダーの活発なエコシステムがあります
- HTML の「オープンソース」構造により、アドインは視覚障害者や失読症の人を支援するためにページの外観を簡単に変更できます
- 「ダークモード」が光過敏症の人のために広くサポートされるようになりました
- 最新の **Web** ブラウザには、言語翻訳などの便利な機能が組み込まれています。
  - これは、あるクラスのユーザーにとっての「アクセシビリティ」の向上です
- 検索エンジンは **HTML** コンテンツでより適切に機能します
  - PDF 内のコンテンツを見つける状況は初期よりもはるかに良くなりましたが
- **HTML**ドキュメントからテキストを簡単に収集
  - arXiv の資料は、今日のほぼすべての大規模言語モデルの重要な部分を占めています



# TeX/LaTeX

- TeX is a computer program that Donald Knuth wrote in the late 1970s to automate the typesetting of his books on the Art of Computer Programming
- Born out of his frustration with the typesetting systems of the times, particularly as it related to mathematics and tables
- TeX is similar to other “text formatters” that existed at the time, such as runoff and Scribe, but was uniquely powerful, in that ...
- TeX allows programming constructs that are powerful enough to make it Turing complete
- This is both a blessing and a curse
  - The blessing is that users can create very sophisticated TeX documents that layout their papers exactly as they wish
  - The curse is that it makes it difficult to re-interpret those papers for a target other than the printed page they were intended for
- TeX は、ドナルドクヌースが1970年代後半に、「Art of Computer Programming」に関する著書の組版を自動化するために作成したプログラムです
- 当時の組版システムの数式やテーブルの貧弱さに対する不満から生まれました
- TeX は、runoff や Scribe など、当時存在していた他の「テキストフォーマッタ」に似ていますが、次の点で独特に強力でした
- TeX は、チューリング完全を満たす、強力なプログラミング言語です
- これは良くもあり、悪くもあります
  - 良しは、ユーザーは論文を思いどおりにレイアウトするととても洗練された TeX ドキュメントを作成できることです
  - 悪しは、論文を組版印刷以外の用法のために再解釈／再利用することが困難になることです

# LaTeX and reinterpretation / LaTeX の再解釈

- TeX's powerful programming features enabled Leslie Lamport to create a package of extensions called LaTeX
- LaTeX defines tags/macros to create structured document
  - Tags look like `\section`, `\subsection`, `\paragraph`
- Almost all scientific documents built with TeX use LaTeX now
- In theory it should be easy to convert LaTeX tags to HTML: `<h1>`, `<h2>`, `<p>`
- In practice most LaTeX papers have additional complexity
- It's another blessing and a curse situation
- Papers in LaTeX almost always include even more packages built on LaTeX that further extend the "language"
- Many of these packages are templates provided by journals or societies so authors can deliver papers formatted according to that journal's standards
- TeX の強力なプログラミング機能により、Leslie Lamport は LaTeX と呼ばれる拡張機能のパッケージを作成しました
- LaTeX は構造化文書を作成するためのタグ/マクロを定義します
  - タグは `\section`、`\subsection`、`\paragraph` などです
- 現在、TeX で作成された大半の論文は LaTeX を使用しています
- 理屈上では、LaTeX タグを HTML に変換するのは容易のはず: `<h1>`、`<h2>`、`<p>`
- 現実では、ほとんどの LaTeX 文書はさらに複雑に
- これは良し／悪し状況の繰り返しです
- LaTeX の論文には、ほとんどの場合 LaTeX 上に構築されたより多くの拡張パッケージが含まれています
- これらのパッケージの多くはジャーナルや学会が提供するテンプレートなので、著者はジャーナルの標準に従ってフォーマットされた論文を提出できます

# LaTeX and reinterpretation / LaTeX の再解釈

- For example, the American Physical Society offers [Physical Review Journals - REVTeX Home Page \(aps.org\)](https://www.aps.org/publications/revtex), built on LaTeX
- A document formatted using REVTeX will be “publication ready” for inclusion in an APS journal
- These templates ease the burden for authors
- But ... there are hundreds, if not thousands of such templates
- Some are provided by large societies, some by small
- Some are just extensions shared amongst individual groups of scientists
- And some eager scientists create extensions just for their own use, sometimes because they want to fine-tune the layout of their papers
  - So things look just right – on a Letter size or A4 page
  - In ways that might look quite wrong in any other medium/format
- 米国物理学会は、LaTeX 上に構築された Physical Review Journals - REVTeX ホームページ (aps.org) を提供しています
- REVTeX を使用してフォーマットされた文書は、APS ジャーナルに掲載できる「出版準備完了」になります
- これらのテンプレートは著者の負担を軽減します
- しかし...そのようなテンプレートは、数千ではないにしても、数百はあります
- 大規模の学会によって提供されるものもあれば、小規模な学会の場合もあります
- 特定の科学者グループ間のみで共有された拡張機能もあります
- 熱心な科学者の中には、論文のレイアウトを微調整したいという理由で、自身で使用するためだけの拡張機能を作成する場合があります
  - US Letterサイズまたは A4 ページではピッタリ
  - 他のメディア/形式ではまったく意味がなくなってしまう時がある

# So what's the problem?

- 90% of arXiv's papers have been submitted in TeX (lately almost all LaTeX) format
- Why can't you just run the TeX compiler to output to HTML instead of PDF?
- Unfortunately, that's not supported, and not easy to support
- Donald Knuth was concerned with the precise typesetting of his technical content
- The TeX compiler he released in 1978 is exclusively intended for that purpose
- Even though LaTeX added structure to the TeX language, that structure is almost completely at compile time when the LaTeX constructs are converted back to TeX primitives
- The core LaTeX team, headed by Frank Mittelbach in Germany, is working on revising TeX/LaTeX processing to preserve this information
  - And add new constructs to LaTeX for things like alt-text
  - See <https://www.latex-project.org/latex3/>
- Currently, their work is
  - exclusively focused on producing better tagged PDF (funded by Adobe)
  - not going to be complete for several more years

# では何が問題か？

- arXiv の論文の 90% は TeX (最近はほぼ全て LaTeX) 形式で提出されています
- TeX コンパイラを実行して PDF ではなく HTML に出力できない理由は？
- 残念ながら、機能はサポートされておらず、サポートするのは難しい
- ドナルド・クヌースは、技術的な内容を正確に組版することに興味を持っていました
- 彼が 1978 年にリリースした TeX コンパイラは、組版に特化しています
- LaTeX は TeX 言語に構造を追加しましたが、その LaTeX の構造はコンパイル時に TeX プリミティブに変換され、失われます
- ドイツの Frank Mittelbach が率いるコア LaTeX チームは、この情報を保存するために TeX/LaTeX 処理の改訂に取り組んでいます
  - そ代替テキストなどのための新しい構造を LaTeX に追加
  - <https://www.latex-project.org/latex3/> を参照
- 現在、彼らの仕事は
  - タグ付き PDF 改善に専念しています (アドビからの資金提供)
  - 数年間は、完成の見込みなし

# But my journal offers HTML now ...

私のジャーナル出版者はHTMLを提供していますが...

- ... and “I gave them the paper in LaTeX”
  - Yes, but ...
  - The process most journals use to create HTML has humans in the loop
  - A tool might be used to get the paper mostly into HTML
  - That tool might be specialized for that journal's LaTeX template
  - And then manual adjustment will be done to make the HTML look right
  - There are a number of service bureaus that do this work (mostly in India)
  - Any process that involves manual labor by anyone other than the authors won't work for arXiv
  - Our volume is just too high – 20,000 papers a month, sometimes 2,000 a day
  - We don't have enough funding to pay for manual adjustments
- ...ちゃんと「LaTeXで書かれた論文を提供しました」
  - そのとおりなのですが...
  - 多くの出版元のHTMLを作成するためのプロセスには手作業が関与しています
  - 論文の大部分をHTMLに取り込むためにツールを使用する余地は確かにあります
  - ツールはしばしば、その出版元のLaTeX テンプレートに特化しています
  - その後、HTML が正しく見えるように手動で調整が行われます。
  - この業務を行うサービス業者が多数あります(主にインド)
  - arXiv側で手作業を伴うプロセスは、arXiv では行えません
  - arXivの扱う論文は多すぎます – 毎月 20,000 件の論文、場合によっては1日 2,000 件の論文
  - 手作業に必要な資金や余裕はarXivにはありません

# arXiv's pragmatic approach    arXiv の実用的なアプローチ

- We didn't want to wait for the LaTeX team to finish its tagging work
  - So we investigated existing tools
  - There have been at least ten attempts to create TeX/LaTeX to HTML tools
  - We had a team of students evaluate all the tools we could find
  - The conclusion was that the best tools were:
    - LaTeXML maintained by Bruce Miller and Deyan Ginev at NIST (National Institute of Standards and Technology)
    - Tex4ht, created by Eitan M. Gurari, now maintained by Michal Hoftich
  - These two tools were roughly tied in the quality of the HTML produced
  - But LaTeXML has a larger library of supported packages and better ongoing support
  - Also the predecessor ar5iv project at arXiv used LaTeXML
- LaTeX チームがタグ付き PDFを完了するまでまてませんでした
  - arXivで既存のツールを調査しました
  - TeX/LaTeX から HTML ツールを作成する試みが少なくとも 10 回ありました
  - arXivは学生のチームに、見つけられるすべてのツールを評価しました
  - 結論として、最適なツールは次のとおりでした。
    - LaTeXML は、NIST (国立標準技術研究所) の Bruce Miller と Deyan Ginev によって保守されています。
    - Tex4ht は Eitan M. Gurari が作者で、現在は Michal Hoftich が保守しています
  - これら 2 つのツールは、生成される HTML の品質においてほぼ同等でした
  - しかし、LaTeXML がサポートしているパッケージの幅が広い ことと、比較的良い継続的な保守があります
  - arXiv の前身の ar5iv プロジェクトでも LaTeXML が使用されていました

# The ar5iv project

- <https://ar5iv.labs.arxiv.org>
- Project started by Dr. Michael Kohlhase from KWARC, and Ph.D. student Deyan Ginev
- Intent was to offer HTML versions for arXiv's entire LaTeX corpus, using LaTeXML
- Mostly succeeded at this, but some 20% failed conversion
- Many others have visual glitches
- As LaTeXML coverage is improved, success rates have increased, glitches decreased
- But old articles must be reconverted to remove glitches
- This is computationally expensive
- Avg \$0.015 per article on Google Cloud ~ \$30,000 for the entire arXiv corpus

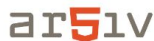

Articles from [arXiv.org](https://arxiv.org) as responsive HTML5 web pages.

Sample: [A Simple Proof of the Quadratic Formula \(1910.06709\)](https://arxiv.org/abs/1910.06709)

View any arXiv article URL by changing the X to a 5

- <https://arxiv.org/abs/1910.06709>
- <https://ar5iv.org/abs/1910.06709>

- <https://ar5iv.labs.arxiv.org>
- KWARC の Michael Kohlhase 博士と博士号学生の Deyan Ginev が ax5iv プロジェクトを開始しました
- 目的は、LaTeXML を使用して、arXiv の LaTeX 資料全体の HTML バージョンを提供することでした
- 多くは成功しましたが、約20% の変換できませんでした
- 見かけがおかしいものも多数あります
- LaTeXML のカバレッジが向上するにつれて、成功率が向上し、不具合は減少しました
- ただし、古い記事は不具合を取り除くために再変換する必要があります
- この処理は計算にコストがかかります
- Google Cloud の記事あたり平均0.015ドル ~ arXiv 資料全体で30,000ドル

レスポンシブ HTML5 Web ページとしての [arxiv.org](https://arxiv.org) の記事

例: 二次方程式の簡単な証明 (1910.06709)

任意の arxiv URL のx を 5 に代えると表示できます

- <https://arxiv.org/abs/1910.06709>
- <https://ar5iv.org/abs/1910.06709>

# The difficulty of converting LaTeX to HTML

## 困難なLaTeX から HTMLへの変換

- LaTeXML, like nearly all the TeX to HTML tools, does not use the actual TeX compiler
  - Because as we said, that compiler in its present state loses structure information
- It therefore does its own processing of the LaTeX documents and packages, and does not attempt to be a full TeX interpreter
  - Because that's really hard and would duplicate the LaTeX team's efforts
- Instead, it includes its own interpretation of the directives
  - It can simply map `\section` to `<h1>`, and the like
  - But, at present, it only executes a subset of the TeX programming constructs
- Instead, most LaTeX packages, and most LaTeX macros have to be “special cased”
  - Perl code (the language of LaTeXML) is written to emulate the TeX construct
- The LaTeXML team has done special case implementations for a few hundred of the most commonly used LaTeXML packages
- LaTeXML は、他の「TeX to HTML」ツールと同様、実際の TeX コンパイラーを使用しません
  - 前述したように、現在の状態のコンパイラでは文書構造情報が失われます
- したがって、LaTeX 文書とパッケージを独自に処理し、完全な TeX インタープリターは諦めています
  - それは本当に難しく、LaTeX チームの努力を二度繰り返すことになるからです
- 代わりに、ディレクティブの独自の解釈が含まれています
  - `\section` を `<h1>` などに単純にマッピングできます。
  - ただし、現時点では TeX 言語構造の一部のみを実行します
- 代わりに、ほとんどの LaTeX パッケージとほとんどのマクロは「特殊ケース」にする必要があります。
  - Perl コード (LaTeXML の言語) は、TeX 構造をエミュレートするために作成されます
- LaTeXML チームは、最も一般的に使用される数百の LaTeXML パッケージに対して特殊ケースの実装を行いました



# Still not complete

# 未完成

- But there is still a long tail of less common packages to be supported
- Not to mention “one-offs” – papers where clever scientists defined their own macros and extensions
- Some popular packages that are hard to implement aren’t yet supported
  - For example, <https://tikz.dev/> – a popular diagramming package
- And there are still some LaTeX constructs that in edge cases don’t render quite right
- So the present results are mostly successful, but with a 20% to 30% error rate
- However, that’s far better than nothing
- And even papers with small glitches are still generally readable
- **Especially for screen readers**
- Something is better than nothing!
- 比較的利用頻度の低い数々のパッケージのサポートが必要です
- 「一回限り」の存在 ー 賢明な科学者が独自のマクロや拡張機能を使用した論文も含まれます
- 実装が難しい一部の人気パッケージはまだサポートされていません
  - たとえば、<https://tikz.dev/> – 人気の図作成パッケージ
- そして、エッジケースでは完全に正しくレンダリングされない LaTeX 構造がまだいくつかあります。
- したがって、現在の結果はおおまかには成功していますが、20% ～ 30% のエラー率があります。
- それでも、全く何もないよりは、はるかに良い状況
- 変換に小さな問題がある論文でも、通常は読むことができます
- **特にスクリーンリーダーの場合**
- 無いよりはマシ！

# Rollout plan for HTML on arXiv

- ar5iv did great work, but few arXiv users knew about it
  - Our present work could be seen as bringing ar5iv “in-house”
- An HTML link will appear on the abstract page for all papers, along with the other links
- The article submission process now creates an HTML version of the paper, alongside the PDF
- Submitters are asked to review the HTML version as part of the submission process
- Submission will not be blocked if the HTML generation fails (unlike the PDF)
- We are hoping that authors will review the HTML rendering and consider making adjustments to their LaTeX source to improve the HTML version
- We also have a prominent “Report Issue” button, so end-users can report HTML rendering issues for us to pass on to the LaTeXML team
- With millions of users performing QA on our HTML, we feel we can improve the conversion process in the future

## Access Paper:

- [Download PDF](#)
- [PostScript](#)
- [Other Formats](#)
- [HTML \(experimental\)](#)

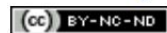

- ar5iv は素晴らしい成果を上げましたが、それをに気づいている arXiv ユーザーはほとんどいませんでした
  - arXiv の現在の取り組みは、ar5iv を「統合」
- すべての抄録ページに HTML リンクが論文その他のリンクと共に表示されます
- 論文の提出プロセスでは 論文のバージョンと PDF に加えて HTML が作成されるようになりました。
- 提出者は、提出プロセスの一環として HTML バージョンを確認するように求められます。
- DF とは違い、HTML の生成が失敗しても提出はブロックされません
- 我々は、作者が HTML レンダリングをレビューし、LaTeX ソースを調整して HTML バージョンを改善することを検討してくれることを期待しています。
- また、突出した「問題を報告」ボタンもあるので、エンドユーザーは HTML レンダリングの問題を報告して、LaTeXML チームに伝えることができます。
- 何百万人ものユーザーが HTML に対して QA を行っているため、将来的には変換プロセスを改善できると考えています。

- Sample HTML paper
- Note the “Experimental” label (「実験的」というラベルに注目してください)
- And the prominent “Report Issue” button, which is screen-reader friendly (スクリーンリーダーに優しい、目立つ「問題を報告」ボタン)
- Or Ctrl-?
- Note that at present we’re only showing new submissions as HTML (現時点では、新しい投稿のみ HTML で表示されていることに注意してください)
- We plan to backfill the historical corpus over time (既存の資料は徐々に変換する予定です)
- In the meantime ar5iv.org is still there (for a while ...) (ar5iv.org はまだしばらくの間存在します)

The screenshot shows a web browser displaying the arXiv Experimental HTML page for the paper "Solution of the Basel problem using the Feynman integral trick" by F. L. Freitas. The page has a red header with the arXiv logo and navigation links. A left sidebar contains a table of contents with links to Introduction, Result, and Conclusion. The main content area includes the title, author information, a date, an abstract, and the start of the introduction section. A "Report Issue" button is visible in the bottom right corner.

License: CC BY 4.0  
arXiv:2312.04608v1 [math.CA] 07 Dec 2023

## Solution of the Basel problem using the Feynman integral trick

F. L. Freitas  
felipolpesfreitas@gmail.com

(Date: December 7, 2023)

### Abstract.

The well known Basel problem, which asks for a closed form expression for the sum of the reciprocals of all perfect squares, together with its solution by Euler in 1734, is one of the most celebrated results of mathematical analysis. In the modern era, numerous proofs of it have been produced, each emphasizing a different style of deduction, as a way of testing the power of some demonstration method. Nevertheless, it's often thought that its solution using calculus involves advanced contour integration techniques or complicated geometric coordinate transformations. We show that this is not the case, as the result can be derived by analyzing basic properties of a particular one-dimensional integral, and as such, can be obtained with techniques typical of regular calculus tests and math competitions.

### 1. Introduction

Solving the Basel problem amounts to proving the following identity:

$$(1) \quad \sum_{n=1}^{\infty} \frac{1}{n^2} = 1 + \frac{1}{2^2} + \frac{1}{3^2} + \frac{1}{4^2} + \dots = \frac{\pi^2}{6}$$

The problem was first solved by Euler in 1734[2]. Ever since his famous original proof, which relied on a generalized Vieta formula for the roots of the function  $\frac{\sin x}{x}$ , numerous other proofs have appeared[3], most emphasizing a different method to the problem.

Report Issue

## Another example, showing

- Dark mode support
- The message the user would see if the paper requires a missing package

## その他の例

- ダークモードのサポート
- 論文に必要なパッケージが不足している場合の表示メッセージ

←

- 1 Introduction
- 2 Related Work
- 3 Guided Flow Matching
- 4 Conditional Generative Modeling
- 5 Planning for Offline RL
- 6 Conclusion

HTML conversions [sometimes display errors](#) due to content that did not convert correctly from the source. This paper uses the following packages that are not yet supported by the HTML conversion tool. Feedback on these issues are not necessary; they are known and are being worked on.

- failed: arydshln

Authors: achieve the best HTML results from your LaTeX submissions by selecting from this list of [supported packages](#).

License: CC BY 4.0

arXiv:2311.13443v2 [cs.LG] 07 Dec 2023

---

**Guided Flows for Generative Modeling and Decision Making**

---

### Abstract

Classifier-free guidance is a key component for enhancing the performance of conditional generative models across diverse tasks. While it has previously demonstrated remarkable improvements for the sample quality, it has only been exclusively employed for diffusion models. In this paper, we integrate classifier-free guidance into Flow Matching (FM) models, an alternative simulation-free approach that trains Continuous Normalizing Flows (CNFs) based on regressing vector fields. We explore the usage of *Guided Flows* for a variety of downstream applications. We show that Guided Flows significantly improves the sample quality in conditional image generation and zero-shot text-to-speech synthesis, boasting state-of-the-art performance. Notably, we are the first to apply

# Acknowledgements

- Kudos to Paul Ginsparg & co. for insisting from the start in 1991 that scientists submit the source code for their papers, instead of just the PDF, which means we can now at least try to convert the 90% of our corpus that is in TeX to HTML.
- We thank the many scientists with disabilities who so generously shared their expertise, insights, and feedback, and guided arXiv's efforts towards impact.

This material is based upon work supported by the National Science Foundation under Award No. OAC-2311521 and by NASA under award No. 20-OSTFL20-0053. Any opinions, findings and conclusions or recommendations expressed in this material are those of the author(s) and do not necessarily reflect the views of the National Science Foundation or of NASA.

- ポール・ギンスパーグとチームに敬意を表します。1991年の当初から、科学者はPDFだけでなく論文のソースコードを提出するよう主張してきました。そのおかげで、少なくともTeXで書かれた資料の90%をHTMLに変換できるようになりました
- 私たちは専門知識、洞察、フィードバックを寛大に共有し、arXivの取り組みを効果に導くよう導いてくださった障害を持つ多くの科学者に感謝します

この資料は、賞番号 OAC-2311521 に基づいて米国科学財団によって支援された研究と、賞番号 20-OSTFL20-0053 に基づいて NASA によって支援された研究に基づいています。この資料に記載されている意見、調査結果、結論または推奨事項は著者のものであり、必ずしも米国科学財団または NASA の見解を反映しているわけではありません。

# Future work

# 今後の取り組み

- Continue to work with the LaTeXML team to improve conversion process
- Figure out a cost-effective way to periodically re-compile the whole corpus to pick up these improvements
- Revisit tooling in a few years when Frank Mittelbach's team is further along
  - We are hopeful that the work to produce tagged PDFs will also enable the generation of HTML output using the core TeX engine
- Future work:
  - Make charts and graphs more accessible
  - Possibly by providing a way for users to access the data behind the graph
  - Auto-caption images and graphs? Presently a challenging AI problem – crowdsourcing may be a better solution
- 引き続き LaTeXML チームと協力して変換プロセスを改善します
- これらの改善点を反映するためにarXivの資料全体を定期的に再コンパイルする費用対効果の高い方法を見つけ出す
- 数年間のうちにFrank Mittelbachのチームが改善したツールを再検討する
  - 私たちは、タグ付きPDFを作成する作業により、コアTeX エンジンを使用したHTML 出力の生成も可能になることを期待しています
- 今後の取り組み:
  - チャートやグラフをよりアクセスしやすくする
  - できればユーザーにグラフの背後にあるデータにアクセスする方法を提供する
  - 画像とグラフの自動キャプション? 現存するAI では困難 – クラウドソーシングがより良い解決策になる可能性があります
