# Supplementary material for: HTML papers on arXiv -- why it is important, and how we made it happen
Source: arXiv:2402.08954 ancillary file (2024-02-14)
Supplement: Supplementary file 2 [file Slide-deck-arXiv-DEIMS-2024.pdf]

# HTML papers on arXiv

Why it's important, and how we make it happen

# arXiv's Importance in Math and Science

- arXiv ([arxiv.org](https://arxiv.org)) is the world's oldest and largest scientific preprint server
- Started in 1991
- Presently housing nearly 2.4 million articles
- Accelerating growth

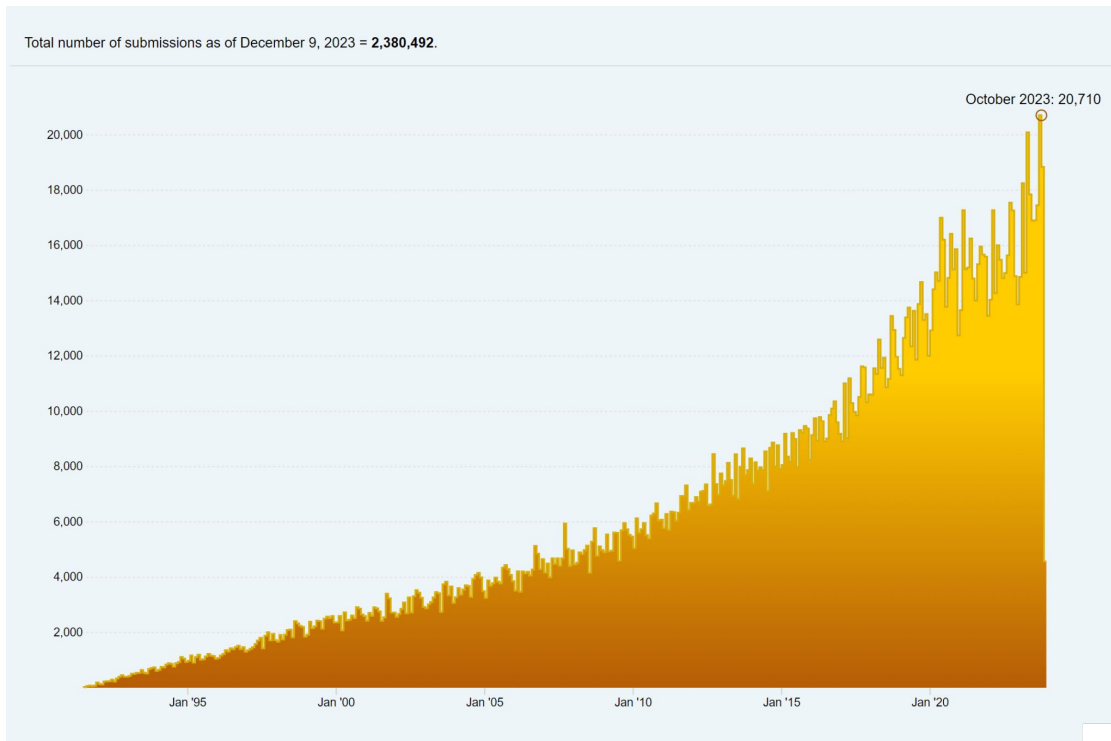

# arXiv's Importance in Math and Science

- In many fields of Physics, Math, and especially Computer Science, cutting edge research is first made available on arXiv. Examples:
  - LLM research ([OpenAI](#), [Deepmind](#), etc.)
  - [LIGO](#) (Gravity wave research; [2017 Nobel Prize in physics](#))
  - Proofs of famous theorems ([Grisha Perelman](#))
- While most papers posted to arXiv are eventually published in journals, in some fields research is often made available only on arXiv
- And even for work subsequently published in journals, early posting to arXiv enables scientists to more rapidly incorporate shared results into new research

# arXiv and accessibility

- Over the past few years, arXiv has made good progress in making <https://arxiv.org> accessible according to [W3C WAI guidelines](#)
- While this allows people with disabilities to more easily access papers, they often cannot read them
- Because arXiv's papers are available almost exclusively in PDF format, which is not, in general, accessible

# PDF limitations - layout

- PDF was originally designed as a digital representation of a printed page
- There is often a mismatch between the paper's geometry and the screen being used to view it
- Zooming in to enlarge the text will often require horizontal scrolling
- “Responsive Design” and reflow are not natural parts of PDF
- Adobe is attempting to address these issues with features like “Liquid Mode”
  - But Liquid Mode is presently mobile-only, and Adobe proprietary
  - Not clear if this retroactive reinterpretation of PDF document layout will work well in all cases
- Improvements in layout and reflow help everyone – not just people with impairments
  - Makes it easier to read papers on mobile devices

# PDF Structure Limitations

- The original structure of the paper, that screen readers often depend on for navigation is typically lost
  - Section headings, captions, links, etc. are reduced to typographic elements like font changes and positioning instructions
  - Mathematical notation in PDF is reduced to symbols and positioning directives
- Adobe introduced tagged PDF in recent years to improve this situation
- But the vast majority of PDF documents in the world are not tagged, tool support has lagged, and there's still the reflow issue
- Again Adobe is attempting to address these issues with features like Tagged PDF
  - arXiv's pipeline from TeX -> PDF currently has poor support for tagged PDF (waiting for the core LaTeX team to give us a solution here)
  - Tagged PDF also has a weak solution for math – display the math as an image and describe the formula in the alt-text for screen readers

# HTML is a better solution

- Designed from the start to render on many devices, arbitrary geometries
- When used correctly preserves structure and intent of the document
- A lot of work has been done to make HTML accessible
- A rich “marketplace” of assistive technologies to make HTML content accessible
- For most people HTML is the gateway to all the content the WWW has to offer
- But ...
- There’s a substantial body of scientific work online available only in PDF format
- Converting PDF content to HTML is challenging, in spite of some interesting work allen.ai has done in this area ([Paper to HTML | Allen Institute for AI](#))
  - Because structure, once lost, is difficult to reconstruct

# HTML has a strong ecosystem

- Because use of the World Wide Web has become fundamental to human existence, a great deal of effort has been expended to make the web accessible
- There's a vibrant ecosystem of screen readers for HTML web pages
- The “open-source” structure of HTML enables add-ins to easily change page appearance to aid visually impaired and people with dyslexia
- “Dark mode” is now widely supported for those with light sensitivities
- Modern web browsers now build-in useful features like language translation
  - Which is an “accessibility” improvement for a class of users
- Search engines function better on HTML content
  - Although the situation for finding content in PDFs is much better now than the early years
- Text harvesting is easily from HTML documents
  - arXiv's corpus is a substantial part of nearly all the Large Language Models today



# TeX/LaTeX

- TeX is a computer program that Donald Knuth wrote in the late 1970s to automate the typesetting of his books on the Art of Computer Programming
- Born out of his frustration with the typesetting systems of the times, particularly as it related to mathematics and tables
- TeX is similar to other “text formatters” that existed at the time, such as runoff and Scribe, but was uniquely powerful, in that ...
- TeX allows programming constructs that are powerful enough to make it Turing complete
- This is both a blessing and a curse
  - The blessing is that users can create very sophisticated TeX documents that layout their papers exactly as they wish
  - The curse is that it makes it difficult to re-interpret those papers for a target other than the printed page they were intended for

# LaTeX and reinterpretation

- TeX's powerful programming features enabled Leslie Lamport to create a package of extensions called LaTeX
- LaTeX defines tags/macros to create structured document
  - Tags look like `\section`, `\subsection`, `\paragraph`
- Almost all scientific documents built with TeX use LaTeX now
- In theory it should be easy to convert LaTeX tags to HTML: `<h1>`, `<h2>`, `<p>`
- In practice most LaTeX papers have additional complexity
- It's another blessing and a curse situation
- Papers in LaTeX almost always include even more packages built on LaTeX that further extend the “language”
- Many of these packages are templates provided by journals or societies so authors can deliver papers formatted according to that journal's standards

# LaTeX and reinterpretation

- For example, the American Physical Society offers [Physical Review Journals - REVTeX Home Page \(aps.org\)](#), built on LaTeX
- A document formatted using REVTeX will be “publication ready” for inclusion in an APS journal
- These templates ease the burden for authors
- But ... there are hundreds, if not thousands of such templates
- Some are provided by large societies, some by small
- Some are just extensions shared amongst individual groups of scientists
- And some eager scientists create extensions just for their own use, sometimes because they want to fine-tune the layout of their papers
  - So things look just right – on a Letter size or A4 page
  - In ways that might look quite wrong in any other medium/format

# So what's the problem?

- 90% of arXiv's papers have been submitted in TeX (lately almost all LaTeX) format
- Why can't you just run the TeX compiler to output to HTML instead of PDF?
- Unfortunately, that's not supported, and not easy to support
- Donald Knuth was concerned with the precise typesetting of his technical content
- The TeX compiler he released in 1978 is exclusively intended for that purpose
- Even though LaTeX added structure to the TeX language, that structure is almost completely at compile time when the LaTeX constructs are converted back to TeX primitives
- The core LaTeX team, headed by Frank Mittelbach in Germany, is working on revising TeX/LaTeX processing to preserve this information
  - And add new constructs to LaTeX for things like alt-text
  - See <https://www.latex-project.org/latex3/>
- Currently, their work is
  - exclusively focused on producing better tagged PDF (funded by Adobe)
  - not going to be complete for several more years

## But my journal offers HTML now ...

- ... and “I gave them the paper in LaTeX”
- Yes, but ...
- The process most journals use to create HTML has humans in the loop
- A tool might be used to get the paper mostly into HTML
- That tool might be specialized for that journal’s LaTeX template
- And then manual adjustment will be done to make the HTML look right
- There are a number of service bureaus that do this work (mostly in India)
- Any process that involves manual labor by anyone other than the authors won’t work for arXiv
- Our volume is just too high – 20,000 papers a month, sometimes 2,000 a day
- We don’t have enough funding to pay for manual adjustments

# arXiv's pragmatic approach

- We didn't want to wait for the LaTeX team to finish its tagging work
- So we investigated existing tools
- There have been at least ten attempts to create TeX/LaTeX to HTML tools
- We had a team of students evaluate all the tools we could find
- The conclusion was that the best tools were:
  - LaTeXML maintained by Bruce Miller and Deyan Ginev at NIST (National Institute of Standards and Technology)
  - Tex4ht, created by Eitan M. Gurari, now maintained by Michal Hoftich
- These two tools were roughly tied in the quality of the HTML produced
- But LaTeXML has a larger library of supported packages and better ongoing support
- Also the predecessor ar5iv project at arXiv used LaTeXML

# The ar5iv project

- <https://ar5iv.labs.arxiv.org>
- Project started by Dr. Michael Kohlhase from KWARC, and Ph.D. student Deyan Ginev
- Intent was to offer HTML versions for arXiv's entire LaTeX corpus, using LaTeXML
- Mostly succeeded at this, but some 20% failed conversion
- Many others have visual glitches
- As LaTeXML coverage is improved, success rates have increased, glitches decreased
- But old articles must be reconverted to remove glitches
- This is computationally expensive
- Avg \$0.015 per article on Google Cloud ~ \$30,000 for the entire arXiv corpus

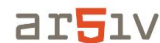

Articles from [arXiv.org](https://arxiv.org) as responsive HTML5 web pages.

Sample: [A Simple Proof of the Quadratic Formula \(1910.06709\)](https://arxiv.org/abs/1910.06709)

View any arXiv article URL by changing the X to a 5

- <https://arxiv.org/abs/1910.06709>
- <https://ar5iv.org/abs/1910.06709>

# The difficulty of converting LaTeX to HTML

- LaTeXML, like nearly all the TeX to HTML tools, does not use the actual TeX compiler
  - Because as we said, that compiler in its present state loses structure information
- It therefore does its own processing of the LaTeX documents and packages, and does not attempt to be a full TeX interpreter
  - Because that's really hard and would duplicate the LaTeX team's efforts
- Instead, it includes its own interpretation of the directives
  - It can simply map `\section` to `<h1>`, and the like
  - But, at present, it only executes a subset of the TeX programming constructs
- Instead, most LaTeX packages, and most LaTeX macros have to be “special cased”
  - Perl code (the language of LaTeXML) is written to emulate the TeX construct
- The LaTeXML team has done special case implementations for a few hundred of the most commonly used LaTeXML packages



# Still not complete

- But there is still a long tail of less common packages to be supported
- Not to mention “one-offs” – papers where clever scientists defined their own macros and extensions
- Some popular packages that are hard to implement aren’t yet supported
  - For example, <https://tikz.dev/> – a popular diagramming package
- And there are still some LaTeX constructs that in edge cases don’t render quite right
- So the present results are mostly successful, but with a 20% to 30% error rate
- However, that’s far better than nothing
- And even papers with small glitches are still generally readable
- **Especially for screen readers**
- Something is better than nothing!

# Rollout plan for HTML on arXiv

- ar5iv did great work, but few arXiv users knew about it
  - Our present work could be seen as bringing ar5iv “in-house”
- An HTML link will appear on the abstract page for all papers, along with the other links
- The article submission process now creates an HTML version of the paper, alongside the PDF
- Submitters are asked to review the HTML version as part of the submission process
- Submission will not be blocked if the HTML generation fails (unlike the PDF)
- We are hoping that authors will review the HTML rendering and consider making adjustments to their LaTeX source to improve the HTML version
- We also have a prominent “Report Issue” button, so end-users can report HTML rendering issues for us to pass on to the LaTeXML team
- With millions of users performing QA on our HTML, we feel we can improve the conversion process in the future

## Access Paper:

- [Download PDF](#)
- [PostScript](#)
- [Other Formats](#)
- [HTML \(experimental\)](#)

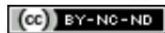

- Sample HTML paper
- Note the “Experimental” label
- And the prominent “Report Issue” button, which is screen-reader friendly
- Or Ctrl-?
- Note that at present we’re only showing new submissions as HTML
- We plan to backfill the historical corpus over time
- In the meantime ar5iv.org is still there (for a while ...)

The screenshot shows a web browser displaying an arXiv HTML paper. The browser's address bar shows the URL `https://browse.arxiv.org/html/2312.04608v1`. The page has a red header with the arXiv logo and text: "This is **Experimental HTML**. We invite you to report rendering errors. Learn more [about this project](#) and [help improve conversions](#)." Navigation links include "Why HTML?", "Report Issue", and "Back to Abstract". A "BETA" badge is visible in the top left of the header.

On the left side of the page, there is a table of contents:

- 1 Introduction
- 2 Result
- 3 Conclusion

The main content area displays the title "Solution of the Basel problem using the Feynman integral trick" and the author "F. L. Freitas" with the email `felipe@freitas@gmail.com`. The license is "CC BY 4.0" and the version is "arXiv:2312.04608v1 [math.CA] 07 Dec 2023". The date "(Date: December 7, 2023)" is also shown.

The **Abstract.** section reads: "The well known Basel problem, which asks for a closed form expression for the sum of the reciprocals of all perfect squares, together with its solution by Euler in 1734, is one of the most celebrated results of mathematical analysis. In the modern era, numerous proofs of it have been produced, each emphasizing a different style of deduction, as a way of testing the power of some demonstration method. Nevertheless, it's often thought that its solution using calculus involves advanced contour integration techniques or complicated geometric coordinate transformations. We show that this is not the case, as the result can be derived by analyzing basic properties of a particular one-dimensional integral, and as such, can be obtained with techniques typical of regular calculus tests and math competitions."

The **1. Introduction** section begins with: "Solving the Basel problem amounts to proving the following identity:"

$$(1) \quad \sum_{n=1}^{\infty} \frac{1}{n^2} = 1 + \frac{1}{2^2} + \frac{1}{3^2} + \frac{1}{4^2} + \dots = \frac{\pi^2}{6}$$

The text continues: "The problem was first solved by Euler in 1734[2]. Ever since his famous original proof, which relied on a generalized Vieta formula for the roots of the function  $\frac{\sin x}{x}$ , numerous other proofs have appeared[3], most emphasizing a different method to the problem."

A red "Report Issue" button is located in the bottom right corner of the page.

## Another example, showing

- Dark mode support
- The message the user would see if the paper requires a missing package

←

1

Introduction

2

Related Work

3

Guided Flow Matching

4

Conditional Generative Modeling

5

Planning for Offline RL

6

Conclusion

HTML conversions [sometimes display errors](#) due to content that did not convert correctly from the source. This paper uses the following packages that are not yet supported by the HTML conversion tool. Feedback on these issues are not necessary; they are known and are being worked on.

• failed: arydshln

Authors: achieve the best HTML results from your LaTeX submissions by selecting from this list of [supported packages](#).

License: CC BY 4.0

arXiv:2311.13443v2 [cs.LG] 07 Dec 2023

Guided Flows for Generative Modeling and Decision Making

Abstract

Classifier-free guidance is a key component for enhancing the performance of conditional generative models across diverse tasks. While it has previously demonstrated remarkable improvements for the sample quality, it has only been exclusively employed for diffusion models. In this paper, we integrate classifier-free guidance into Flow Matching (FM) models, an alternative simulation-free approach that trains Continuous Normalizing Flows (CNFs) based on regressing vector fields. We explore the usage of *Guided Flows* for a variety of downstream applications. We show that Guided Flows significantly improves the sample quality in conditional image generation and zero-shot text-to-speech synthesis, boasting state-of-the-art performance. Notably, we are the first to apply

# Acknowledgements

- Kudos to Paul Ginsparg & co. for insisting from the start in 1991 that scientists submit the source code for their papers, instead of just the PDF, which means we can now at least try to convert the 90% of our corpus that is in TeX to HTML.
- We thank the many scientists with disabilities who so generously shared their expertise, insights, and feedback, and guided arXiv's efforts towards impact.

This material is based upon work supported by the National Science Foundation under Award No.~OAC-2311521. Any opinions, findings and conclusions or recommendations expressed in this material are those of the author(s) and do not necessarily reflect the views of the National Science Foundation.

# Future work

- Continue to work with the LaTeXML team to improve conversion process
- Figure out a cost-effective way to periodically re-compile the whole corpus to pick up these improvements
- Revisit tooling in a few years when Frank Mittelbach's team is further along
  - We are hopeful that the work to produce tagged PDFs will also enable the generation of HTML output using the core TeX engine
- Future work:
  - Make charts and graphs more accessible
  - Possibly by providing a way for users to access the data behind the graph
  - Auto-caption images and graphs? Presently a challenging AI problem – crowdsourcing may be a better solution
